# Supplementary material for: Emergence of collective dynamical chirality for achiral active particles
Source: arXiv:1610.00114 source file (2017-02-14)
Supplement: Supplementary file 1 [file SI.pdf]

# Supplemental Information: Emergence of collective dynamical chirality for achiral active particles

Huijun Jiang, Huai Ding, Mingfeng Pu, Zhonghuai Hou
*Department of Chemical Physics & Hefei National Laboratory for Physical Sciences at Microscales, iChEM, University of Science and Technology of China, Hefei, Anhui 230026, China*

## I. DETAILS OF THE LATTICE BOLTZMANN METHOD

The hydrodynamic interaction between active particles is realized by Lattice-Boltzmann method[1]. The lattice Boltzmann equation(LBE) with a force and white noise can be written as

$$f_i(\mathbf{x}+\mathbf{e}_i\Delta t, t+\Delta t) - f_i(\mathbf{x},t) = -\frac{1}{\tau}\left[f_i(\mathbf{x},t) - f_i^{eq}(\mathbf{x},t)\right] + F_i\Delta t + f_i'(\mathbf{x},t) \tag{1}$$

where $f_i(\mathbf{x},t)$ is the distribution function for fluid particles with velocity $\mathbf{e}_i$ at position $\mathbf{x}$ and time $t$, $\Delta t$ is the time increment and in our work we set $\Delta t = 1$. $f_i^{eq}$ is the equilibrium distribution function and $\tau$ is the relaxation time. $f'$ represents the fluctuation induced by the thermal motion of the fluid's particles.

The fluid density $\rho$ and velocity $\mathbf{u}$ are read

$$\begin{aligned}\rho &= \textstyle\sum_i f_i \\ \rho\mathbf{u} &= \textstyle\sum_i \mathbf{e}_i f_i\end{aligned} \tag{2}$$

In the two-dimension space, we use the Q2D9 model to divide the space. Therefore, the velocities of the fluid particles are defined by $\mathbf{e}_0 = (0,0)$, $\mathbf{e}_i = (\cos[\pi(i-1)/2], \sin[\pi(i-1)/2])\,c$ for $i = 1 \sim 4$, $\mathbf{e}_i = \sqrt{2}(\cos[\pi(i-9/2)/2], \sin[\pi(i-9/2)/2])\,c$ for $i = 5 \sim 8$, with $c = \Delta x/\Delta t = 1$. The equilibrium distribution function is $f_i^{eq} = \omega_i\rho\left[1 + 3(\mathbf{e}_i\cdot\mathbf{u})/c_s^2 + 9(\mathbf{e}_i\cdot\mathbf{u})^2/2c_s^4 - 3\mathbf{u}^2/2c_s^2\right]$ for the incompressible model, where $\omega_0 = 4/9$, $\omega_i = 1/9$ for $i = 1,2,3,4$ and $\omega_i = 1/36$ for $i = 5,6,7,8$, and $c_s = 1/\sqrt{3}$ is the sound speed of the model.

In Eq.1, $F_i$ is a function of the force exerting on the fluid. There are many models of $F_i$. The form of $F_i$ we used in our paper is

$$F_i = \omega_i\rho\left[\frac{\mathbf{e}_i - \mathbf{u}}{c_s^2} + \frac{(\mathbf{e}_i\cdot\mathbf{u})\,\mathbf{e}_i}{c_s^4}\right]\cdot\mathbf{F} \tag{3}$$

where $\mathbf{F}$ is the force exerting on the fluid. Due to the low mach number of system studied here, collision of the fluid particles on the confinement boundary is considered as non-slip, which is realized by using the bounce-back scheme.

Notice that, active particles are smaller than the lattice spacing, indicating that the surface between active particles and the fluid is also smaller than the lattice spacing. So that, we can treat the active particles as point-like particles as that has been reported in literature[2]. We use the LBE-Lagrange approach to describe the motion of point-like particles in fluid flow. The main force that the fluid exerts on the 2D-particles[3] in low Reynolds is

$$\mathbf{F}_d = \frac{32}{3}\eta a\,(\mathbf{u} - \mathbf{u}_p)$$

where $a$ is the radius of active particles, $\mathbf{u}_p$ is the velocity of active particles and $\mathbf{u}$ the flow velocity in the position of these particles. Therefore, the reaction force exerting on the fluid is $\mathbf{F} = -\,\mathbf{F}_d$. We distribute this force on the four lattice points surrounding the active particle by linear interpolation.

In Eq.1, $f_i'$ represents the fluctuation induced by thermal motion of the fluid's particles[4]. It satisfies the mass and momentum conservation

$$\begin{aligned}\textstyle\sum_i f_i' &= 0 \\ \textstyle\sum_i f_i'\mathbf{e}_i &= \mathbf{0}\end{aligned} \tag{4}$$

$$\begin{aligned} f_0' = 0, f_1' = f_3' &= \frac{1}{2\tau}\sigma'_{yy}, f_2' = f_4' = \frac{1}{2\tau}\sigma'_{xx} \\ f_5' = f_7' &= -\frac{1}{4\tau}\left[\sigma'_{xx} + \sigma'_{yy} + \sigma'_{xy}\right] \\ f_6' = f_8' &= -\frac{1}{4\tau}\left[\sigma'_{xx} + \sigma'_{yy} - \sigma'_{yy}\right]\end{aligned} \tag{5}$$

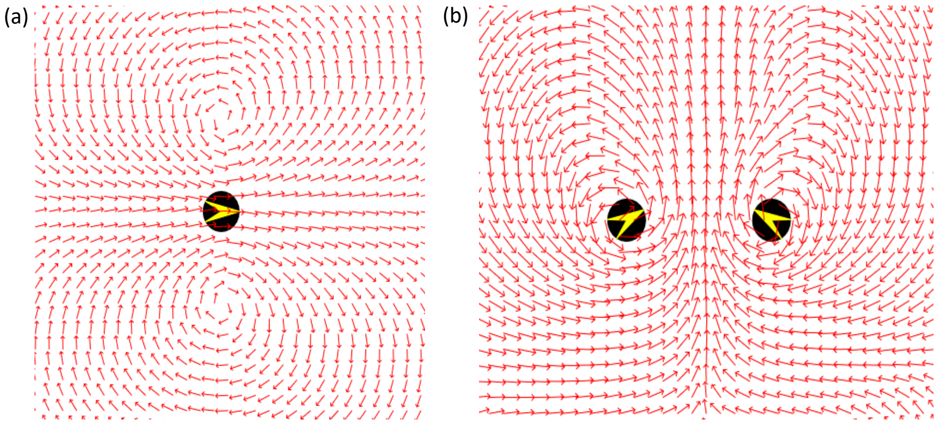


FIG. S1: Active force induced flow field for (a) a single particle and (b) two interacting particles.

and the random stress should satisfy the following conditions

$$\begin{aligned} \left\langle \sigma'_{\alpha\beta} \right\rangle &= 0 \\ \left\langle \sigma'_{\alpha\beta}\left(\mathbf{x}_1, t_1\right) \sigma'_{\gamma\delta}\left(\mathbf{x}_2, t_2\right) \right\rangle &= 2\eta k_B T \left[\delta_{\alpha\gamma}\delta_{\beta\delta} + \delta_{\alpha\delta}\delta_{\beta\gamma}\right] \delta\left(\mathbf{x}_1 - \mathbf{x}_2\right) \delta\left(t_1 - t_2\right) \end{aligned} \tag{6}$$

When a point-like active particle is put in the fluctuation system, the random stress should be derived from the fluctuation-dissipation relationship. Thus, similar as that in Ref.5, the method is modified by adding a stochastic term $\mathbf{f}$ in the motion equation of point-like particles. Hereto, we construct a basic fluid model to study the collective chirality dynamics.

## II. ACTIVITY INUDUCED FLOW FIELD

Flow field for a single particle and for two interacting particles is shown in Fig.S1(a) and (b), respectively. To illustrate clearly the effect of the active force on the flow field, the noise part and the confinement are neglected, and the position of particles are fixed. As expected, each particles are force monopoles, while for two interacting particles, the flow field leads to an effective alignment of their orientation.

## III. EFFECT OF IMMERSED BOUNDARY

Notice that the active particles we considered are point-like. To find out the effect of explicit particle boundary, we have repeated simulations for larger disk particles with immersed boundary realized by smoothed-profile method. In the method, the surface of the colloid is treated as an interface in which a kind of fluid with infinite viscosity is constructed, and the viscosity has a smooth change in the surface. The technical details of this method has been published in Ref.6. By applying this method to the same system as we mentioned above, similar formation of CDC has also been observed. Since a larger lattice is needed to model the fluid for active particles with immersed boundary, we choose the point-like particles instead to facilitate numerical calculations. Moreover, since active particles are point-like, the torque that flow exerts on them are not considered. In our opinion, CDC may be easier to be observed if torque is included.

[1] Shiyi Chen and Gary D. Doolen. Lattice boltzmann method for fluid flows. *Annu. Rev. Fluid Mech.*, 30:329–64, 1998.
[2] O. Filippova and D. Hänel. Lattice-boltzmann simulation of gas-particle flow in filters. *Computers & Fluids*, 26:697–712, 1997.
[3] Ruben van Drongelen, Anshuman Pal, Carl P. Goodrich, and Timon Idema. Collective dynamics of soft active particles. *Phys. Rev. E*, 91:032706, 2015.
[4] Anthony J. C. Ladd. Numerical simulations of particulate suspensions via a discretized boltzmann equation part i. theoretical foundation. *Journal of Fluid Mechanics*, 271:285–309, 1994.

[5] Patrick Ahlrichs and Burkhard Dünweg. Lattice-boltzmann simulation of polymer-solvent systems. *Int. J. Mod. Phys. C*, 09:1429, 1998.

[6] Jafari, Saeed and Yamamoto, Ryoichi and Rahnama, Mohamad. Lattice-Boltzmann method combined with smoothed-profile method for particulate suspensions. *Phys. Rev. E*, 83:026702, 2011.
